# Supplementary material for: Making Reliable and Flexible Decisions in Long-tailed Classification
Source: arXiv:2501.14090 source file (2025-01-23)
Supplement: Supplementary file 1 [file a_decision_loss.tex]

\bl{This section is moved to the main body.}

As mentioned in the paper, we design the decision gain to be the following:
\begin{equation}
    g(d|\bm{x},\bm{\theta}):=\prod_{y'}p(y'|\bm{x},\bm{\theta})^{U_{y',d}}.
    \label{A1}
\end{equation}
Our design is different from previous work like~\citet{cobb2018loss}, which uses
\begin{equation}
    g'(d|\bm{x},\bm{\theta}):=\sum_{y'}U_{y',d}\cdot p(y'|\bm{x},\bm{\theta}).
    \label{A2}
\end{equation}
Both definitions achieve the goal of averaging the predictive probability $p(y|\bm{x},\bm{\theta})$ weighted by the utility values. However, our design has two advantages: \romannumeral1) Stability: Eq.~\ref{A1} is more stable for training. After taking the logarithm, Eq.~\ref{A1} becomes $\sum_{y'}U_{y',d(\bm{x})}\cdot\log p(y'|\bm{x},\bm{\theta})$ which is a weighted average of the log probabilities, while Eq.~\ref{A2} becomes $\log\sum_{y'}U_{y',d(\bm{x})}\cdot p(y'|\bm{x},\bm{\theta})$, which is a log of weighted average of the probabilities and not commonly used in classification problems. \romannumeral2) Flexibility: Eq.~\ref{A1} allows for more general and flexible utility values whereas Eq.~\ref{A2} requires the utility matrix $\bm{U}$ to be positive definite (otherwise we may not be able to compute the logarithm in Eq.~\ref{A2}). Due to these reasons, we use Eq.~\ref{A1} in this paper.
